# Supplementary material for: Measuring geometric phase without interferometry
Source: arXiv:1805.10381 source file (2018-05-25)
Supplement: Supplementary file 1 [file Berry-phase_SupMat.pdf]

# Supplemental Material: Measuring geometric phase without interferometry

T. Malhotra,[1,2] R. Gutiérrez-Cuevas,[2,3] J. Hassett,[2,3] M. R. Dennis,[4,5] A. N. Vamivakas,[1,2,3,6,*] and M. A. Alonso[2,3,7,†]

[1]*Department of Physics, University of Rochester, Rochester, New York 14627, USA*
[2]*Center for Coherence and Quantum Optics, University of Rochester, Rochester, NY 14627, USA*
[3]*The Institute of Optics, University of Rochester, Rochester, NY 14627, USA*
[4]*H. H. Wills Physics Laboratory, University of Bristol, Bristol BS8 1TL, UK*
[5]*School of Physics and Astronomy, University of Birmingham, Birmingham B15 2TT, UK*
[6]*Materials Science, University of Rochester, Rochester, New York 14627, USA*
[7]*Aix Marseille Université, Centrale Marseille, Institut Fresnel, UMR 7249, 13397 Marseille Cedex 20, France*

## I. THEORY

Structured Gaussian beams can be described in terms of a continuous two-parameter family of rays. Each ray within the family is identified by a pair of values of the periodic variables $\tau$ and $\eta$ as

$$\boldsymbol{Q}(\tau,\eta) = Q_0 \Re\left\{\boldsymbol{v}[\theta(\eta),\phi(\eta)]e^{-\mathrm{i}(\tau-\tau_0)}\right\}, \tag{S1a}$$

$$\boldsymbol{P}(\tau,\eta) = P_0 \Im\left\{\boldsymbol{v}[\theta(\eta),\phi(\eta)]e^{-\mathrm{i}(\tau-\tau_0)}\right\}, \tag{S1b}$$

where $\boldsymbol{Q}$ gives the transverse position of the rays and $\boldsymbol{P}$ their transverse direction cosines, $Q_0$ sets the size of the beam [so that the fundamental Gaussian has waist width $w_0 = Q_0/(N+1)^{1/2}$] and $P_0 = (N+1)\lambda/Q_0$ gives the beam's angular divergence, with $\lambda$ being the wavelength and $N$ the total order [1]. In these equations, the reference value $\tau_0$ for the variable $\tau$ can be chosen freely and may depend on $\eta$, and $\boldsymbol{v}$ is the analog to the Jones vector used in polarization and is defined as

$$\boldsymbol{v}(\theta,\phi) = \cos\frac{\theta}{2}\left(\cos\frac{\phi}{2},\sin\frac{\phi}{2}\right) + \mathrm{i}\sin\frac{\theta}{2}\left(-\sin\frac{\phi}{2},\cos\frac{\phi}{2}\right), \tag{S2}$$

with $-\pi/2 \leq \theta \leq \pi/2$ and $0 \leq \phi < 2\pi$ corresponding to latitude and longitude over the Poincaré sphere.

As can be seen from Eqs. (S1), both the transverse position and direction cosines of the ray trace an ellipse as $\tau$ varies. The angles $\theta$ and $\phi$ are parametrized in terms of the second parameter, $\eta$, in order to trace a curve over the modal Poincaré sphere (MPS) referred to here as the Poincaré path (PP) [1]. For the case of the Hermite-Gauss (HG), Laguerre-Gauss (LG) and the more general Hermite-Laguerre-Gauss (HLG) [2] modes considered in this work, the shape of the PP is a circle whose center is the modal spot used in the standard MPS representations [3, 4]. The solid angle subtended by the PP is quantized according to $\Omega = 2\pi(2n+1)/(N+1)$ with $n = 0, 1, ..., \lfloor N/2 \rfloor$ as shown in [1, 5]. For a given $n$, the LG modes have azimuthal orders $l = \pm(N-2n)$, while the rotated HG modes along the equator have orders $m$ and $n$ with $m = N - n \geq n$. That is, for any given $N$, larger PP circles lead to LG modes with more radial structure and smaller vorticity, and to HG modes with smaller aspect ratios. Therefore, modes with different $n$ are supported by the same MPS as long as they have the same total order $N$.

Given an HG mode for which the modal spot is along the equator (i.e. the PP is contained in a plane perpendicular to the equatorial plane), one can arrive at a particularly convenient parametrization of the rays given by [1]

$$\boldsymbol{Q} = Q_0\left[c_m\cos(\tau-\eta/2), c_n\cos(\tau+\eta/2)\right], \tag{S3a}$$

$$\boldsymbol{P} = -P_0\left[c_m\sin(\tau-\eta/2), c_n\sin(\tau+\eta/2)\right], \tag{S3b}$$

with $c_s = \sqrt{(2s+1)}/2(N+1)$. This mode can be transformed by using an anamorphic, rotated fractional Fourier transform (ARfFT) [6, 7] whose effect is a rotation over the MPS. This transformation belongs to a wider class of linear canonical transformations (LCT), all of which are represented by $4\times4$ symplectic matrices [7, 8]. In the ray domain, the effect of the system is modeled by multiplying the four-vector $(Q_x, Q_y, P_x, P_y)^\intercal$ by this matrix. The symplectic matrix representation of the ARfFT is

$$F_\theta(\alpha_x,\alpha_y) = R(\theta)F(\alpha_x,\alpha_y)R(-\theta), \tag{S4}$$

where

$$F(\alpha_x,\alpha_y) = \begin{pmatrix} \cos\alpha_x & 0 & \sin\alpha_x & 0 \\ 0 & \cos\alpha_y & 0 & \sin\alpha_y \\ -\sin\alpha_x & 0 & \cos\alpha_x & 0 \\ 0 & -\sin\alpha_y & 0 & \cos\alpha_y \end{pmatrix} \tag{S5}$$

is the matrix representation of a separable anamorphic fractional Fourier transform (AfFT) and

$$R(\theta) = \begin{pmatrix} \cos\theta & \sin\theta & 0 & 0 \\ -\sin\theta & \cos\theta & 0 & 0 \\ 0 & 0 & \cos\theta & \sin\theta \\ 0 & 0 & -\sin\theta & \cos\theta \end{pmatrix} \tag{S6}$$

is the matrix representing physical rotations. [The angles $\alpha_x$ and $\alpha_y$ are the same as those in Eq. (4) in the main

* nick.vamivakas@rochester.edu
† miguel.alonso@rochester.edu

text.] In the wave domain, the ARfFT results from the use of this matrix on the LCT (or Collins) formula [7, 8].

We consider closed trajectories traced by the modal spot, resulting from a sequence of ARfFTs like the one depicted in Fig. 2 of the main text, in which the modal spot moves from the equator to the north pole along a meridian, then down to the south pole via a second meridian at an angle $\gamma$ with respect to the first, and finally back to the initial point along the initial meridian. The matrix for this closed loop, found through the concatenation of its three parts, takes a simple form:

$$F_{\frac{\pi}{4}}\left(\frac{\pi}{8},-\frac{\pi}{8}\right)F_{\frac{\pi}{4}+\frac{\gamma}{2}}\left(-\frac{\pi}{4},\frac{\pi}{4}\right)F_{\frac{\pi}{4}}\left(\frac{\pi}{8},-\frac{\pi}{8}\right)=F(\gamma,-\gamma), \tag{S7}$$

which is just an AfFT aligned with the Cartesian axes. This comes as no surprise since HG modes are eigenfunctions of such AfFT. Since the fFT can describe the evolution of a 1D quantum harmonic oscillator [9], the AfFT above can be written in terms of harmonic-oscillator Hamiltonian operators in the form of Eqs. (1) and (2) in the main text. The eigenvalues of this transformation provide the geometric phase gained along the curve, which is given by $(N-2n)\gamma$. Using the results presented in [10], relating the centroid of a fractional Fourier transform to that of the original function and its Fourier transform, we arrive at Eq. (3) in the main text. Notice also that the application of this matrix to the ray family in Eq. (S3) indeed results in the same ray family except for the shift $\eta \to \eta - 2\gamma$.

Notice that the Gouy phase also corresponds to a fFT, but one with equal parameters $F(\xi,\xi)$, where $\xi = (N+1)\zeta/N$ [11]. Here, again, by applying the corresponding matrix to the ray family [Eq. (S3)] we obtain the same rays but with the parameter $\tau$ shifted by $\zeta$. This makes it easy to implement alongside the PB phase: they can both be modeled by a single fFT with matrix representation $F(\xi+\gamma,\xi-\gamma)$, thus leading to the result presented in Eq. (5) in the main text.

## II. EXPERIMENT

Details of the calibration of the interferometric measurements are now given. The complete HG mode (without obstructions) is sent through both the test and reference arms. A piston phase $\psi$ (varying between 0 and $2\pi$) is implemented on SLM2, and the power resulting from the interference from both arms is recorded by a bucket detector as a function of $\psi$. The interferometer is path-stabilized (see [12] for details) to ensure that the two arms of the interferometer remain in a fixed path-difference configuration during the data acquisition. We use as a reference an interference measurement resulting from using the set-up in the inverted imaging mode (that is, using $\alpha_x = \alpha_y = \pi$) to deduce the phases corresponding to different values of $\gamma$. The negative branch of the arccosine function was chosen for $\alpha > \pi$ in order to match the measured interferometric PB phase. The interferograms are fitted with sinusoids to recover the phase, and the phase of the reference measurements (which include an extra phase of $\pi$ due to the image inversion) is subtracted, leading to the desired PB phase.


[1] M. A. Alonso and M. R. Dennis, Optica **4**, 476 (2017).
[2] E. G. Abramochkin and V. G. Volostnikov, J. Opt. A: Pure Appl. Opt. **6**, S157 (2004).
[3] M. J. Padgett and J. Courtial, Opt. Lett. **24**, 430 (1999).
[4] S. J. Habraken and G. Nienhuis, Opt. Lett. **35**, 3535 (2010).
[5] M. R. Dennis and M. A. Alonso, Phil. Trans. R. Soc. A **375**, 20150441 (2017).
[6] J. A. Rodrigo, T. Alieva, and M. L. Calvo, J. Opt. Soc. Am. A **23**, 2494 (2006).
[7] T. Alieva and M. J. Bastiaans, Opt. Lett. **32**, 1226 (2007).
[8] J. J. Healy, M. A. Kutay, H. M. Ozaktas, and J. T. Sheridan, *Linear canonical transforms: Theory and applications* (Springer, 2015).
[9] G. Agarwal and R. Simon, Opt. Commun. **110**, 23 (1994).
[10] M. J. Bastiaans and T. Alieva, EURASIP J. Appl. Signal Process. **2005**, 1535 (2005).
[11] H. M. Ozaktas and D. Mendlovic, Opt. Lett. **19**, 1678 (1994).
[12] T. Malhotra, W. E. Farriss, J. Hassett, A. F. Abouraddy, J. R. Fienup, and A. N. Vamivakas, Opt. Express **26**, 8719 (2018).
